# Supplementary material for: Confidence Calibration and Predictive Uncertainty Estimation for Deep Medical Image Segmentation
Source: arXiv:1911.13273 source file (2020-06-29)
Supplement: Supplementary file 1 [file appendix.tex]

\clearpage
\section{Quantitative Results}

Figure \ref{fig:drawing_brain} visually compares the baselines trained with cross entropy, Dice loss with those calibrated with ensembling and through some representative examples over the three segmentation tasks.
For each prediction map, a reliability diagram over the whole volume is provided.

\begin{figure*}[h]
% todo: remove vspace later
% \vspace{-0.6cm}
\centering
% {\includegraphics[scale=0.5]{figures/drawing.eps}}
\setlength{\tabcolsep}{1pt}
\begin{tabular}{lcccccc}
  %\includegraphics[width=21mm]{figures/figure_3/figure3_4.pdf} &
  %&
  %\includegraphics[width=21mm]{figures/figure_3/figure3_4.pdf} &
  %&
  %\includegraphics[width=21mm]{figures/figure_3/figure3_8.pdf} &
  %&
  %\includegraphics[width=21mm]{figures/figure_3/figure3_0.pdf} &
  %\\
\parbox[t]{4mm}{\rotatebox[origin=l]{90}{\small{$~~~~~~{\mathcal{L}_{CE}}$}}} &
\includegraphics[width=25mm]{figures/figure_3/figure3_5.pdf} &
\includegraphics[width=26mm]{figures/figure_3/figure3_5_reliability_diagram.pdf} &
\includegraphics[width=25mm]{figures/figure_3/figure3_5.pdf} &
\includegraphics[width=26mm]{figures/figure_3/figure3_5_reliability_diagram.pdf} &
\includegraphics[width=25mm]{figures/figure_3/figure3_9.pdf} &
\includegraphics[width=26mm]{figures/figure_3/figure3_9_reliability_diagram.pdf}\\

\parbox[t]{4mm}{\rotatebox[origin=l]{90}{\small{$~~{\mathcal{L}_{CE}~(EN)}$}}} &
\includegraphics[width=25mm]{figures/figure_3/figure3_5.pdf} &
\includegraphics[width=26mm]{figures/figure_3/figure3_5_reliability_diagram.pdf} &
\includegraphics[width=25mm]{figures/figure_3/figure3_5.pdf} &
\includegraphics[width=26mm]{figures/figure_3/figure3_5_reliability_diagram.pdf} &
\includegraphics[width=25mm]{figures/figure_3/figure3_9.pdf} &
\includegraphics[width=26mm]{figures/figure_3/figure3_9_reliability_diagram.pdf}\\

\parbox[t]{4mm}{\rotatebox[origin=l]{90}{\small{$~~~~~~{\mathcal{L}_{DSC}}$}}} &
\includegraphics[width=25mm]{figures/figure_3/figure3_5.pdf} &
\includegraphics[width=26mm]{figures/figure_3/figure3_5_reliability_diagram.pdf} &
\includegraphics[width=25mm]{figures/figure_3/figure3_5.pdf} &
\includegraphics[width=26mm]{figures/figure_3/figure3_5_reliability_diagram.pdf} &
\includegraphics[width=25mm]{figures/figure_3/figure3_9.pdf} &
\includegraphics[width=26mm]{figures/figure_3/figure3_9_reliability_diagram.pdf}\\

\parbox[t]{4mm}{\rotatebox[origin=l]{90}{\small{$~~~~{MCDO}$}}} &
\includegraphics[width=25mm]{figures/figure_3/figure3_5.pdf} &
\includegraphics[width=26mm]{figures/figure_3/figure3_5_reliability_diagram.pdf} &
\includegraphics[width=25mm]{figures/figure_3/figure3_5.pdf} &
\includegraphics[width=26mm]{figures/figure_3/figure3_5_reliability_diagram.pdf} &
\includegraphics[width=25mm]{figures/figure_3/figure3_9.pdf} &
\includegraphics[width=26mm]{figures/figure_3/figure3_9_reliability_diagram.pdf}\\

\parbox[t]{4mm}{\rotatebox[origin=l]{90}{\small{$~~{\mathcal{L}_{DSC}~(EN)}$}}} &
\includegraphics[width=25mm]{figures/figure_3/figure3_5.pdf} &
\includegraphics[width=26mm]{figures/figure_3/figure3_5_reliability_diagram.pdf} &
\includegraphics[width=25mm]{figures/figure_3/figure3_5.pdf} &
\includegraphics[width=26mm]{figures/figure_3/figure3_5_reliability_diagram.pdf} &
\includegraphics[width=25mm]{figures/figure_3/figure3_9.pdf} &
\includegraphics[width=26mm]{figures/figure_3/figure3_9_reliability_diagram.pdf}\\

  %\small{Ground Truth}&
  %\multicolumn{2}{c}{\small{Baseline ($\mathcal{L}_{CE}$)}} & 
  %\multicolumn{2}{c}{\small{Baseline ($\mathcal{L}_{DSC}$)}} & 
  %\multicolumn{2}{c}{\small{Ensemble (M=50)}} \\
\end{tabular}
\caption{
Examples of uncertainty estimation quality of baselines trained with cross entropy loss, Dice loss, and models calibrated with ensembling.
Calibration has been applied only to models trained with Dice loss.
MRI images are overlaid with class probabilities, and reliability diagrams (together with ECE\%, NLL, and Brier score) are given for that specific volume.
In the reliability diagrams only the bins with greater than 1000 samples are shown.
Top, middle, and bottom rows show the results for non-enhancing tumor, the right ventricle, and the prostate gland segmentation tasks, respectively.
The color bar for the class probability values is given in Figure
\ref{fig:introduction}.
}
\label{fig:drawing_brain}
\end{figure*}

\begin{figure*}[h]
	\centering
	% {\includegraphics[scale=0.5]{figures/drawing.eps}}
	\setlength{\tabcolsep}{1pt}
	\begin{tabular}{lcccccc}
		%\includegraphics[width=21mm]{figures/figure_3/figure3_4.pdf} &
		%&
		%\includegraphics[width=21mm]{figures/figure_3/figure3_4.pdf} &
		%&
		%\includegraphics[width=21mm]{figures/figure_3/figure3_8.pdf} &
		%&
		%\includegraphics[width=21mm]{figures/figure_3/figure3_0.pdf} &
		%\\
		\parbox[t]{4mm}{\rotatebox[origin=l]{90}{\small{$~~~~~~{\mathcal{L}_{CE}}$}}} &
		\includegraphics[width=25mm]{figures/figure_3/figure3_5.pdf} &
		\includegraphics[width=26mm]{figures/figure_3/figure3_5_reliability_diagram.pdf} &
		\includegraphics[width=25mm]{figures/figure_3/figure3_5.pdf} &
		\includegraphics[width=26mm]{figures/figure_3/figure3_5_reliability_diagram.pdf} &
		\includegraphics[width=25mm]{figures/figure_3/figure3_9.pdf} &
		\includegraphics[width=26mm]{figures/figure_3/figure3_9_reliability_diagram.pdf}\\
		
		\parbox[t]{4mm}{\rotatebox[origin=l]{90}{\small{$~~{\mathcal{L}_{CE}~(EN)}$}}} &
		\includegraphics[width=25mm]{figures/figure_3/figure3_5.pdf} &
		\includegraphics[width=26mm]{figures/figure_3/figure3_5_reliability_diagram.pdf} &
		\includegraphics[width=25mm]{figures/figure_3/figure3_5.pdf} &
		\includegraphics[width=26mm]{figures/figure_3/figure3_5_reliability_diagram.pdf} &
		\includegraphics[width=25mm]{figures/figure_3/figure3_9.pdf} &
		\includegraphics[width=26mm]{figures/figure_3/figure3_9_reliability_diagram.pdf}\\
		
		\parbox[t]{4mm}{\rotatebox[origin=l]{90}{\small{$~~~~~~{\mathcal{L}_{DSC}}$}}} &
		\includegraphics[width=25mm]{figures/figure_3/figure3_5.pdf} &
		\includegraphics[width=26mm]{figures/figure_3/figure3_5_reliability_diagram.pdf} &
		\includegraphics[width=25mm]{figures/figure_3/figure3_5.pdf} &
		\includegraphics[width=26mm]{figures/figure_3/figure3_5_reliability_diagram.pdf} &
		\includegraphics[width=25mm]{figures/figure_3/figure3_9.pdf} &
		\includegraphics[width=26mm]{figures/figure_3/figure3_9_reliability_diagram.pdf}\\
		
		\parbox[t]{4mm}{\rotatebox[origin=l]{90}{\small{$~~~~{MCDO}$}}} &
		\includegraphics[width=25mm]{figures/figure_3/figure3_5.pdf} &
		\includegraphics[width=26mm]{figures/figure_3/figure3_5_reliability_diagram.pdf} &
		\includegraphics[width=25mm]{figures/figure_3/figure3_5.pdf} &
		\includegraphics[width=26mm]{figures/figure_3/figure3_5_reliability_diagram.pdf} &
		\includegraphics[width=25mm]{figures/figure_3/figure3_9.pdf} &
		\includegraphics[width=26mm]{figures/figure_3/figure3_9_reliability_diagram.pdf}\\
		
		\parbox[t]{4mm}{\rotatebox[origin=l]{90}{\small{$~~{\mathcal{L}_{DSC}~(EN)}$}}} &
		\includegraphics[width=25mm]{figures/figure_3/figure3_5.pdf} &
		\includegraphics[width=26mm]{figures/figure_3/figure3_5_reliability_diagram.pdf} &
		\includegraphics[width=25mm]{figures/figure_3/figure3_5.pdf} &
		\includegraphics[width=26mm]{figures/figure_3/figure3_5_reliability_diagram.pdf} &
		\includegraphics[width=25mm]{figures/figure_3/figure3_9.pdf} &
		\includegraphics[width=26mm]{figures/figure_3/figure3_9_reliability_diagram.pdf}\\
		
		%\small{Ground Truth}&
		%\multicolumn{2}{c}{\small{Baseline ($\mathcal{L}_{CE}$)}} & 
		%\multicolumn{2}{c}{\small{Baseline ($\mathcal{L}_{DSC}$)}} & 
		%\multicolumn{2}{c}{\small{Ensemble (M=50)}} \\
	\end{tabular}
	\caption{
		Examples of uncertainty estimation quality of baselines trained with cross entropy loss, Dice loss, and models calibrated with ensembling.
		Calibration has been applied only to models trained with Dice loss.
		MRI images are overlaid with class probabilities, and reliability diagrams (together with ECE\%, NLL, and Brier score) are given for that specific volume.
		In the reliability diagrams only the bins with greater than 1000 samples are shown.
		Top, middle, and bottom rows show the results for non-enhancing tumor, the right ventricle, and the prostate gland segmentation tasks, respectively.
		The color bar for the class probability values is given in Figure
		\ref{fig:introduction}.
	}
	\label{fig:drawing_heart}
\end{figure*}

\begin{figure*}[h]
	% todo: remove vspace later
	% \vspace{-0.6cm}
	\centering
	% {\includegraphics[scale=0.5]{figures/drawing.eps}}
	\setlength{\tabcolsep}{1pt}
	\begin{tabular}{lcccccc}
		%\includegraphics[width=21mm]{figures/figure_3/figure3_4.pdf} &
		%&
		%\includegraphics[width=21mm]{figures/figure_3/figure3_4.pdf} &
		%&
		%\includegraphics[width=21mm]{figures/figure_3/figure3_8.pdf} &
		%&
		%\includegraphics[width=21mm]{figures/figure_3/figure3_0.pdf} &
		%\\
		\parbox[t]{4mm}{\rotatebox[origin=l]{90}{\small{$~~~~~~{\mathcal{L}_{CE}}$}}} &
		\includegraphics[width=25mm]{figures/figure_3/figure3_5.pdf} &
		\includegraphics[width=26mm]{figures/figure_3/figure3_5_reliability_diagram.pdf} &
		\includegraphics[width=25mm]{figures/figure_3/figure3_5.pdf} &
		\includegraphics[width=26mm]{figures/figure_3/figure3_5_reliability_diagram.pdf} &
		\includegraphics[width=25mm]{figures/figure_3/figure3_9.pdf} &
		\includegraphics[width=26mm]{figures/figure_3/figure3_9_reliability_diagram.pdf}\\
		
		\parbox[t]{4mm}{\rotatebox[origin=l]{90}{\small{$~~{\mathcal{L}_{CE}~(EN)}$}}} &
		\includegraphics[width=25mm]{figures/figure_3/figure3_5.pdf} &
		\includegraphics[width=26mm]{figures/figure_3/figure3_5_reliability_diagram.pdf} &
		\includegraphics[width=25mm]{figures/figure_3/figure3_5.pdf} &
		\includegraphics[width=26mm]{figures/figure_3/figure3_5_reliability_diagram.pdf} &
		\includegraphics[width=25mm]{figures/figure_3/figure3_9.pdf} &
		\includegraphics[width=26mm]{figures/figure_3/figure3_9_reliability_diagram.pdf}\\
		
		\parbox[t]{4mm}{\rotatebox[origin=l]{90}{\small{$~~~~~~{\mathcal{L}_{DSC}}$}}} &
		\includegraphics[width=25mm]{figures/figure_3/figure3_5.pdf} &
		\includegraphics[width=26mm]{figures/figure_3/figure3_5_reliability_diagram.pdf} &
		\includegraphics[width=25mm]{figures/figure_3/figure3_5.pdf} &
		\includegraphics[width=26mm]{figures/figure_3/figure3_5_reliability_diagram.pdf} &
		\includegraphics[width=25mm]{figures/figure_3/figure3_9.pdf} &
		\includegraphics[width=26mm]{figures/figure_3/figure3_9_reliability_diagram.pdf}\\
		
		\parbox[t]{4mm}{\rotatebox[origin=l]{90}{\small{$~~~~{MCDO}$}}} &
		\includegraphics[width=25mm]{figures/figure_3/figure3_5.pdf} &
		\includegraphics[width=26mm]{figures/figure_3/figure3_5_reliability_diagram.pdf} &
		\includegraphics[width=25mm]{figures/figure_3/figure3_5.pdf} &
		\includegraphics[width=26mm]{figures/figure_3/figure3_5_reliability_diagram.pdf} &
		\includegraphics[width=25mm]{figures/figure_3/figure3_9.pdf} &
		\includegraphics[width=26mm]{figures/figure_3/figure3_9_reliability_diagram.pdf}\\
		
		\parbox[t]{4mm}{\rotatebox[origin=l]{90}{\small{$~~{\mathcal{L}_{DSC}~(EN)}$}}} &
		\includegraphics[width=25mm]{figures/figure_3/figure3_5.pdf} &
		\includegraphics[width=26mm]{figures/figure_3/figure3_5_reliability_diagram.pdf} &
		\includegraphics[width=25mm]{figures/figure_3/figure3_5.pdf} &
		\includegraphics[width=26mm]{figures/figure_3/figure3_5_reliability_diagram.pdf} &
		\includegraphics[width=25mm]{figures/figure_3/figure3_9.pdf} &
		\includegraphics[width=26mm]{figures/figure_3/figure3_9_reliability_diagram.pdf}\\
		
		%\small{Ground Truth}&
		%\multicolumn{2}{c}{\small{Baseline ($\mathcal{L}_{CE}$)}} & 
		%\multicolumn{2}{c}{\small{Baseline ($\mathcal{L}_{DSC}$)}} & 
		%\multicolumn{2}{c}{\small{Ensemble (M=50)}} \\
	\end{tabular}
	\caption{
		Examples of uncertainty estimation quality of baselines trained with cross entropy loss, Dice loss, and models calibrated with ensembling.
		Calibration has been applied only to models trained with Dice loss.
		MRI images are overlaid with class probabilities, and reliability diagrams (together with ECE\%, NLL, and Brier score) are given for that specific volume.
		In the reliability diagrams only the bins with greater than 1000 samples are shown.
		Top, middle, and bottom rows show the results for non-enhancing tumor, the right ventricle, and the prostate gland segmentation tasks, respectively.
		The color bar for the class probability values is given in Figure
		\ref{fig:introduction}.
	}
	\label{fig:drawing_prostate}
\end{figure*}

\clearpage
\section{Number of Models}
\TK{The three graphs in} Figure \ref{fig:n_ensembles} show\st{s} \TK{the quantitative\st{the}} improvement in \TK{the}  calibration and segmentation as a function of the number of models in the ensemble, \TK{\st{M} for each of the three segmentation applications of the prostate, the heart, and the brain tumors. The images in the figure qualitatively illustrate this improvement for the prostate gland segmentation task.}
\TK{\st{As we see, for the prostate, the heart, and the brain tumor segmentation, using even five ensembles (M=5) can reduce the NLL by about $66\%$, $44\%$, and $62\%$, respectively.}}

\begin{figure*}[h]
\centering
%\vspace{-2cm}
\begin{tabular}{lllllll}
	\includegraphics[width=20mm,height=18mm]{figures/figure_2/figure2_0.pdf}
	\includegraphics[width=18mm]{figures/figure_2/figure2_1.pdf}
	\includegraphics[width=18mm]{figures/figure_2/figure2_2.pdf}
	\includegraphics[width=18mm]{figures/figure_2/figure2_2.pdf}
	\includegraphics[width=18mm]{figures/figure_2/figure2_2.pdf}
	\includegraphics[width=18mm]{figures/figure_2/figure2_2.pdf}
	\includegraphics[width=18mm]{figures/figure_2/figure2_3.pdf}\\
	\includegraphics[width=20mm,height=18mm]{figures/figure_2/figure2_4.pdf}
	\includegraphics[width=18mm]{figures/figure_2/figure2_5.pdf}
	\includegraphics[width=18mm]{figures/figure_2/figure2_6.pdf}
	\includegraphics[width=18mm]{figures/figure_2/figure2_6.pdf}
	\includegraphics[width=18mm]{figures/figure_2/figure2_6.pdf}
	\includegraphics[width=18mm]{figures/figure_2/figure2_6.pdf}
	\includegraphics[width=20mm,height=18mm]{figures/figure_2/figure2_7.pdf}\\
	\includegraphics[width=20mm,height=18mm]{figures/figure_2/figure2_4.pdf}
	\includegraphics[width=18mm]{figures/figure_2/figure2_5.pdf}
	\includegraphics[width=18mm]{figures/figure_2/figure2_6.pdf}
	\includegraphics[width=18mm]{figures/figure_2/figure2_6.pdf}
	\includegraphics[width=18mm]{figures/figure_2/figure2_6.pdf}
	\includegraphics[width=18mm]{figures/figure_2/figure2_6.pdf}
	\includegraphics[width=20mm,height=18mm]{figures/figure_2/figure2_7.pdf}\\
\end{tabular}

\begin{tabular}{lllllll}
	\includegraphics[width=20mm,height=18mm]{figures/figure_2/figure2_0.pdf}
	\includegraphics[width=18mm]{figures/figure_2/figure2_1.pdf}
	\includegraphics[width=18mm]{figures/figure_2/figure2_2.pdf}
	\includegraphics[width=18mm]{figures/figure_2/figure2_2.pdf}
	\includegraphics[width=18mm]{figures/figure_2/figure2_2.pdf}
	\includegraphics[width=18mm]{figures/figure_2/figure2_2.pdf}
	\includegraphics[width=18mm]{figures/figure_2/figure2_3.pdf}\\
		\includegraphics[width=20mm,height=18mm]{figures/figure_2/figure2_4.pdf}
	\includegraphics[width=18mm]{figures/figure_2/figure2_5.pdf}
	\includegraphics[width=18mm]{figures/figure_2/figure2_6.pdf}
	\includegraphics[width=18mm]{figures/figure_2/figure2_6.pdf}
	\includegraphics[width=18mm]{figures/figure_2/figure2_6.pdf}
	\includegraphics[width=18mm]{figures/figure_2/figure2_6.pdf}
	\includegraphics[width=20mm,height=18mm]{figures/figure_2/figure2_7.pdf}\\
	\includegraphics[width=20mm,height=18mm]{figures/figure_2/figure2_4.pdf}
	\includegraphics[width=18mm]{figures/figure_2/figure2_5.pdf}
	\includegraphics[width=18mm]{figures/figure_2/figure2_6.pdf}
	\includegraphics[width=18mm]{figures/figure_2/figure2_6.pdf}
	\includegraphics[width=18mm]{figures/figure_2/figure2_6.pdf}
	\includegraphics[width=18mm]{figures/figure_2/figure2_6.pdf}
	\includegraphics[width=20mm,height=18mm]{figures/figure_2/figure2_7.pdf}\\
\end{tabular}

\begin{tabular}{lllllll}
	\includegraphics[width=20mm,height=18mm]{figures/figure_2/figure2_0.pdf}
	\includegraphics[width=18mm]{figures/figure_2/figure2_1.pdf}
	\includegraphics[width=18mm]{figures/figure_2/figure2_2.pdf}
	\includegraphics[width=18mm]{figures/figure_2/figure2_2.pdf}
	\includegraphics[width=18mm]{figures/figure_2/figure2_2.pdf}
	\includegraphics[width=18mm]{figures/figure_2/figure2_2.pdf}
	\includegraphics[width=18mm]{figures/figure_2/figure2_3.pdf}\\
		\includegraphics[width=20mm,height=18mm]{figures/figure_2/figure2_4.pdf}
	\includegraphics[width=18mm]{figures/figure_2/figure2_5.pdf}
	\includegraphics[width=18mm]{figures/figure_2/figure2_6.pdf}
	\includegraphics[width=18mm]{figures/figure_2/figure2_6.pdf}
	\includegraphics[width=18mm]{figures/figure_2/figure2_6.pdf}
	\includegraphics[width=18mm]{figures/figure_2/figure2_6.pdf}
	\includegraphics[width=20mm,height=18mm]{figures/figure_2/figure2_7.pdf}\\
	\includegraphics[width=20mm,height=18mm]{figures/figure_2/figure2_4.pdf}
	\includegraphics[width=18mm]{figures/figure_2/figure2_5.pdf}
	\includegraphics[width=18mm]{figures/figure_2/figure2_6.pdf}
	\includegraphics[width=18mm]{figures/figure_2/figure2_6.pdf}
	\includegraphics[width=18mm]{figures/figure_2/figure2_6.pdf}
	\includegraphics[width=18mm]{figures/figure_2/figure2_6.pdf}
	\includegraphics[width=20mm,height=18mm]{figures/figure_2/figure2_7.pdf}\\
\end{tabular}
\caption{
qualitative example shows T2-weighted MRI images of the prostate gland at different axial positions (apex - left column, mid-gland - middle two columns, and base - right column) overlaid with color-coded prostate probability map. The overlaid probability map in the middle row shows the results of inference for an ensemble of size M=2, and the bottom row for M=50. White line shows the ground truth boundary of the prostate. Qualitative improvement in segmentation and uncertainty estimation is obvious.
}
\label{fig:n_ensembles_dice}
\end{figure*}

\begin{figure*}[h]
	\centering
	%\vspace{-2cm}
	\begin{tabular}{lllllll}
		\includegraphics[width=20mm,height=18mm]{figures/figure_2/figure2_0.pdf}
		\includegraphics[width=18mm]{figures/figure_2/figure2_1.pdf}
		\includegraphics[width=18mm]{figures/figure_2/figure2_2.pdf}
		\includegraphics[width=18mm]{figures/figure_2/figure2_2.pdf}
		\includegraphics[width=18mm]{figures/figure_2/figure2_2.pdf}
		\includegraphics[width=18mm]{figures/figure_2/figure2_2.pdf}
		\includegraphics[width=18mm]{figures/figure_2/figure2_3.pdf}\\
		\includegraphics[width=20mm,height=18mm]{figures/figure_2/figure2_4.pdf}
		\includegraphics[width=18mm]{figures/figure_2/figure2_5.pdf}
		\includegraphics[width=18mm]{figures/figure_2/figure2_6.pdf}
		\includegraphics[width=18mm]{figures/figure_2/figure2_6.pdf}
		\includegraphics[width=18mm]{figures/figure_2/figure2_6.pdf}
		\includegraphics[width=18mm]{figures/figure_2/figure2_6.pdf}
		\includegraphics[width=20mm,height=18mm]{figures/figure_2/figure2_7.pdf}\\
		\includegraphics[width=20mm,height=18mm]{figures/figure_2/figure2_4.pdf}
		\includegraphics[width=18mm]{figures/figure_2/figure2_5.pdf}
		\includegraphics[width=18mm]{figures/figure_2/figure2_6.pdf}
		\includegraphics[width=18mm]{figures/figure_2/figure2_6.pdf}
		\includegraphics[width=18mm]{figures/figure_2/figure2_6.pdf}
		\includegraphics[width=18mm]{figures/figure_2/figure2_6.pdf}
		\includegraphics[width=20mm,height=18mm]{figures/figure_2/figure2_7.pdf}\\
	\end{tabular}
	
	\begin{tabular}{lllllll}
		\includegraphics[width=20mm,height=18mm]{figures/figure_2/figure2_0.pdf}
		\includegraphics[width=18mm]{figures/figure_2/figure2_1.pdf}
		\includegraphics[width=18mm]{figures/figure_2/figure2_2.pdf}
		\includegraphics[width=18mm]{figures/figure_2/figure2_2.pdf}
		\includegraphics[width=18mm]{figures/figure_2/figure2_2.pdf}
		\includegraphics[width=18mm]{figures/figure_2/figure2_2.pdf}
		\includegraphics[width=18mm]{figures/figure_2/figure2_3.pdf}\\
		\includegraphics[width=20mm,height=18mm]{figures/figure_2/figure2_4.pdf}
		\includegraphics[width=18mm]{figures/figure_2/figure2_5.pdf}
		\includegraphics[width=18mm]{figures/figure_2/figure2_6.pdf}
		\includegraphics[width=18mm]{figures/figure_2/figure2_6.pdf}
		\includegraphics[width=18mm]{figures/figure_2/figure2_6.pdf}
		\includegraphics[width=18mm]{figures/figure_2/figure2_6.pdf}
		\includegraphics[width=20mm,height=18mm]{figures/figure_2/figure2_7.pdf}\\
		\includegraphics[width=20mm,height=18mm]{figures/figure_2/figure2_4.pdf}
		\includegraphics[width=18mm]{figures/figure_2/figure2_5.pdf}
		\includegraphics[width=18mm]{figures/figure_2/figure2_6.pdf}
		\includegraphics[width=18mm]{figures/figure_2/figure2_6.pdf}
		\includegraphics[width=18mm]{figures/figure_2/figure2_6.pdf}
		\includegraphics[width=18mm]{figures/figure_2/figure2_6.pdf}
		\includegraphics[width=20mm,height=18mm]{figures/figure_2/figure2_7.pdf}\\
	\end{tabular}
	
	\begin{tabular}{lllllll}
		\includegraphics[width=20mm,height=18mm]{figures/figure_2/figure2_0.pdf}
		\includegraphics[width=18mm]{figures/figure_2/figure2_1.pdf}
		\includegraphics[width=18mm]{figures/figure_2/figure2_2.pdf}
		\includegraphics[width=18mm]{figures/figure_2/figure2_2.pdf}
		\includegraphics[width=18mm]{figures/figure_2/figure2_2.pdf}
		\includegraphics[width=18mm]{figures/figure_2/figure2_2.pdf}
		\includegraphics[width=18mm]{figures/figure_2/figure2_3.pdf}\\
		\includegraphics[width=20mm,height=18mm]{figures/figure_2/figure2_4.pdf}
		\includegraphics[width=18mm]{figures/figure_2/figure2_5.pdf}
		\includegraphics[width=18mm]{figures/figure_2/figure2_6.pdf}
		\includegraphics[width=18mm]{figures/figure_2/figure2_6.pdf}
		\includegraphics[width=18mm]{figures/figure_2/figure2_6.pdf}
		\includegraphics[width=18mm]{figures/figure_2/figure2_6.pdf}
		\includegraphics[width=20mm,height=18mm]{figures/figure_2/figure2_7.pdf}\\
		\includegraphics[width=20mm,height=18mm]{figures/figure_2/figure2_4.pdf}
		\includegraphics[width=18mm]{figures/figure_2/figure2_5.pdf}
		\includegraphics[width=18mm]{figures/figure_2/figure2_6.pdf}
		\includegraphics[width=18mm]{figures/figure_2/figure2_6.pdf}
		\includegraphics[width=18mm]{figures/figure_2/figure2_6.pdf}
		\includegraphics[width=18mm]{figures/figure_2/figure2_6.pdf}
		\includegraphics[width=20mm,height=18mm]{figures/figure_2/figure2_7.pdf}\\
	\end{tabular}
	\caption{
		\textbf{Improvements in calibration and segmentation as a function of the number of models in the ensemble.} Top row: calibration quality in terms of NLL as number of models $M$ increases for prostate, heart, and brain tumor segmentation.
		Red line shows the mean and the shaded area 95\% CI for NLL.
		The NLL for model trained with cross entropy (within bounding boxes) is  shown as a gray dot.
		For each task an ensemble of size M=10 outperforms the model trained with cross entropy in terms of NLL.
		Middle and bottom rows: a qualitative example shows T2-weighted MRI images of the prostate gland at different axial positions (apex - left column, mid-gland - middle two columns, and base - right column) overlaid with color-coded prostate probability map. The overlaid probability map in the middle row shows the results of inference for an ensemble of size M=2, and the bottom row for M=50. White line shows the ground truth boundary of the prostate. Qualitative improvement in segmentation and uncertainty estimation is obvious.
	}
	\label{fig:n_ensembles_ce}
\end{figure*}

\clearpage
\newpage
\section{Segment-level Predictive Uncertainty}
{\color{lightgray}\blindtext[1]}

\begin{figure*}[h]
	\centering
	\setlength{\tabcolsep}{1pt}
	\begin{tabular}{ccccccccc}
		\includegraphics[width=18mm,height=17.8mm]{figures/figure_4/figure4w_4.pdf} &
		\includegraphics[width=18mm]{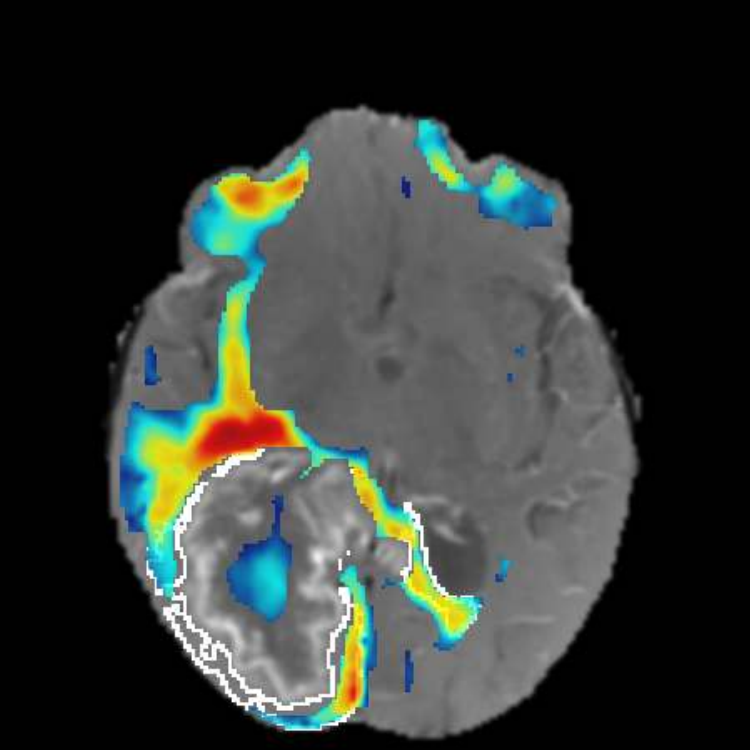} &
		\includegraphics[width=18mm]{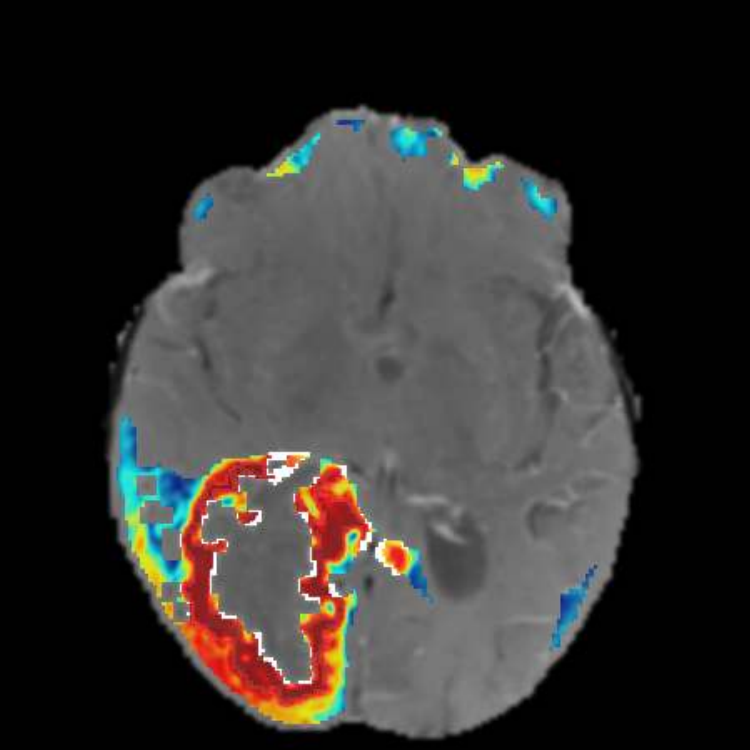} &
		\includegraphics[width=18mm]{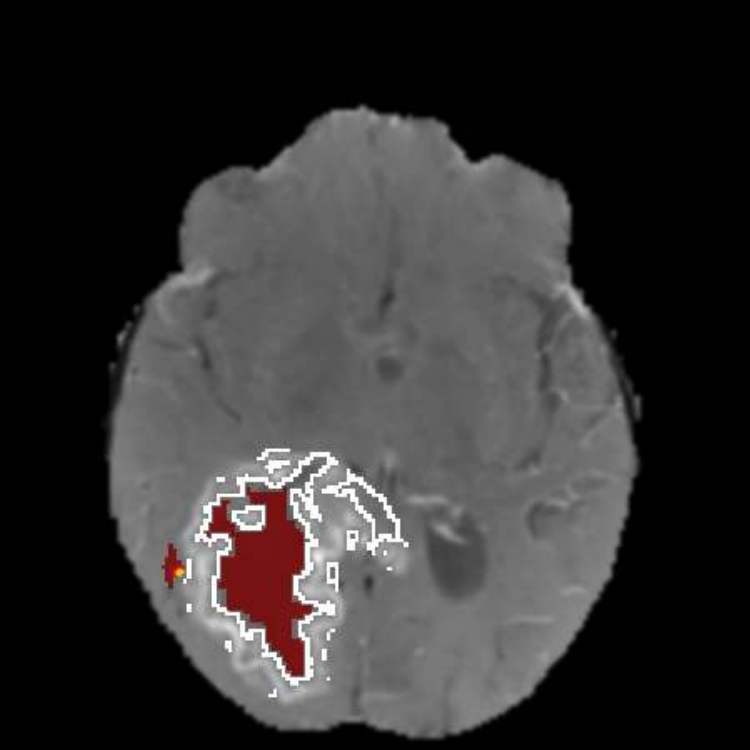} &
		\includegraphics[width=18mm]{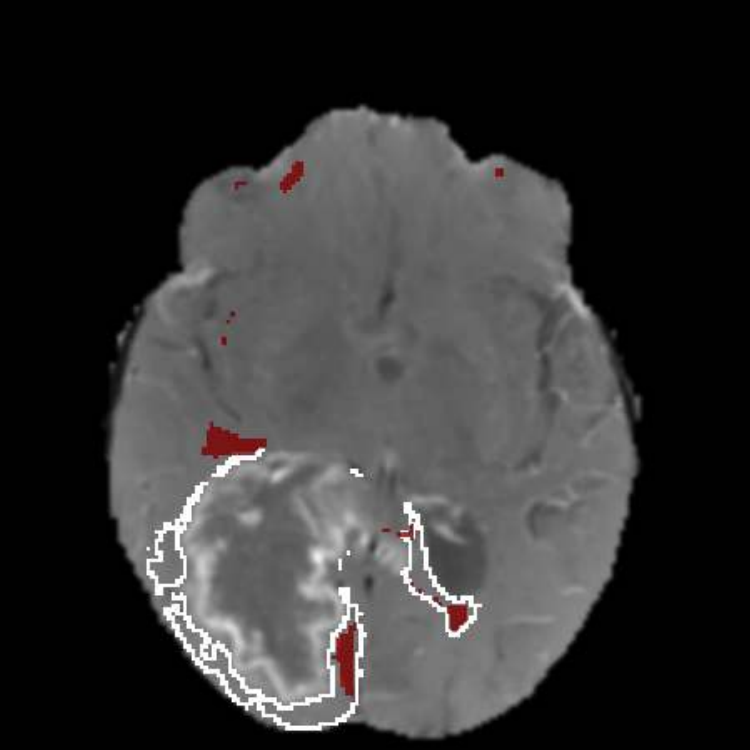} &
		\includegraphics[width=18mm]{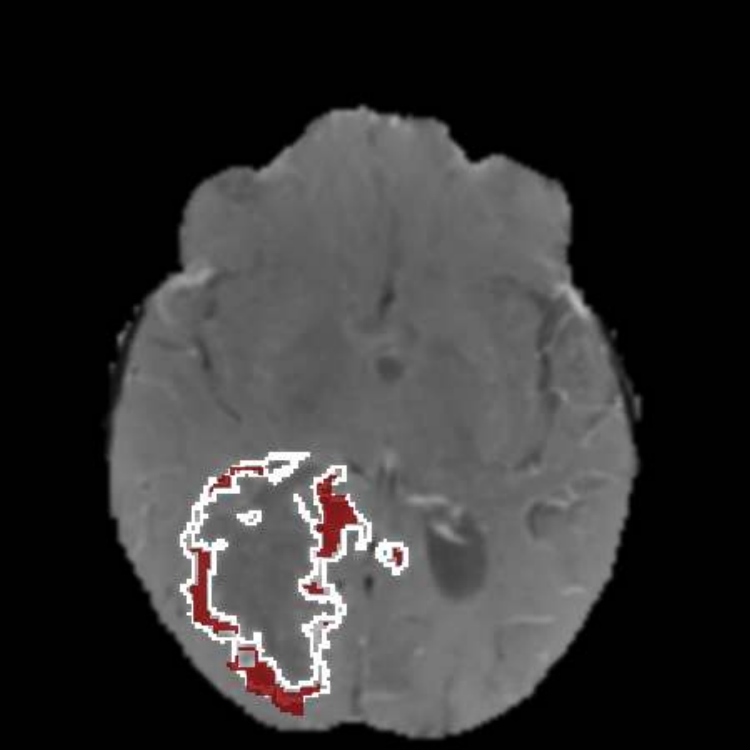} &
		\includegraphics[width=18mm]{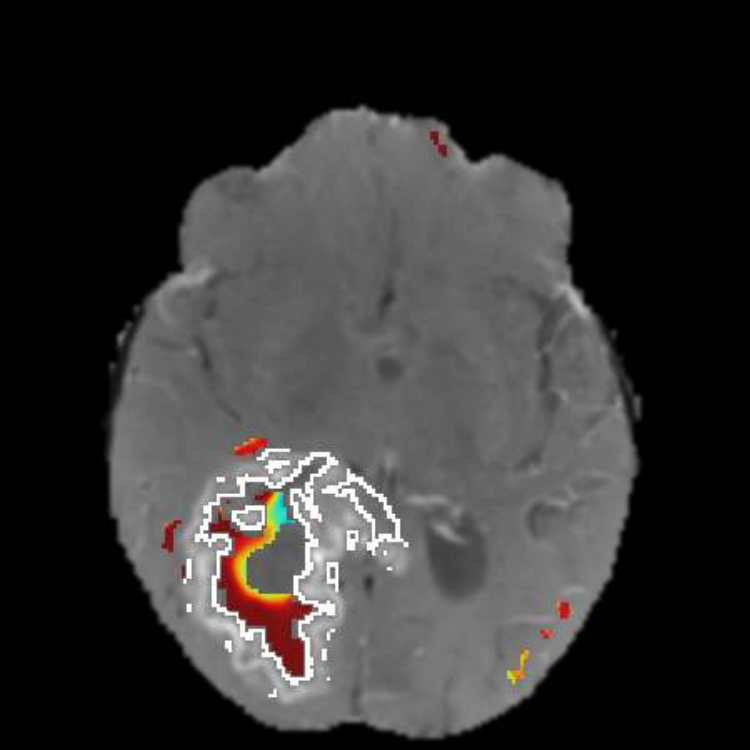} &
		\includegraphics[width=18mm]{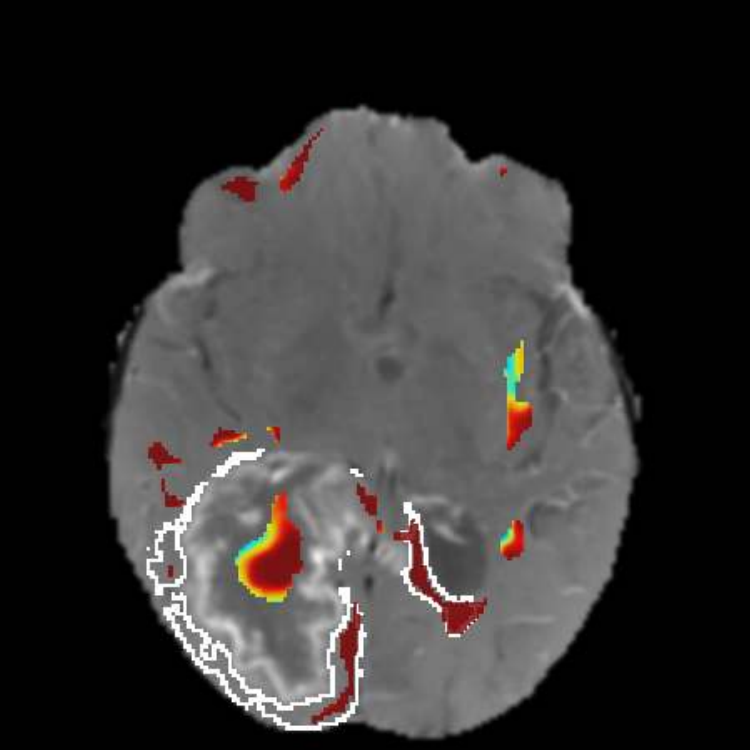} &
		\includegraphics[width=27mm, height=18mm]{figures/figure_4/figure4_20.pdf} \\
		\includegraphics[width=18mm,height=17.8mm]{figures/figure_4/figure4w_12.pdf} &
		\includegraphics[width=18mm]{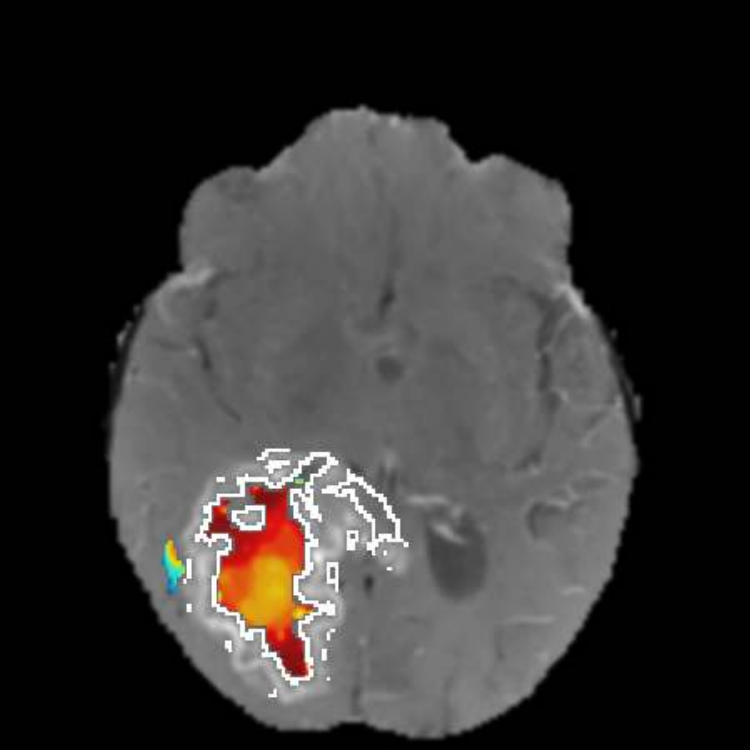} &
		\includegraphics[width=18mm]{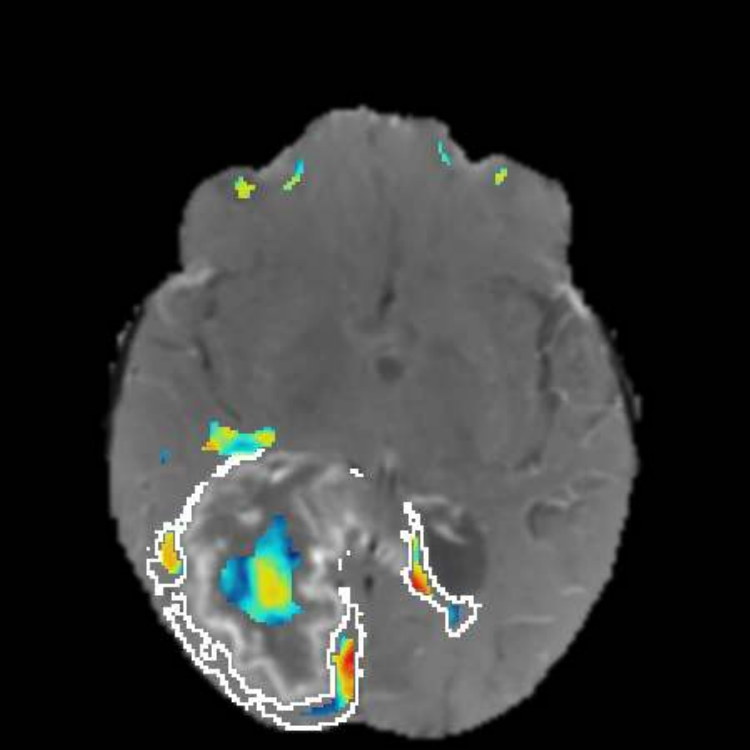} &
		\includegraphics[width=18mm]{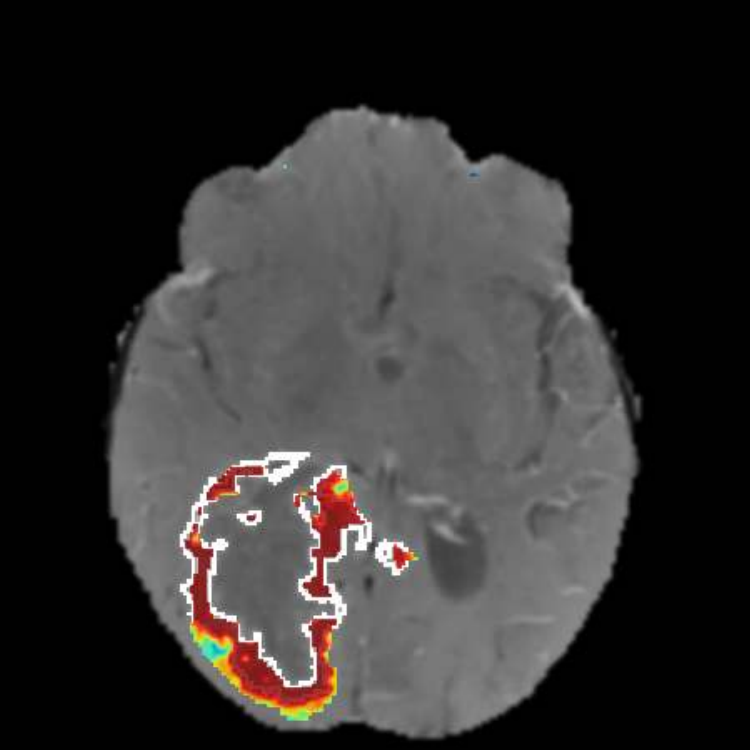} &
		\includegraphics[width=18mm]{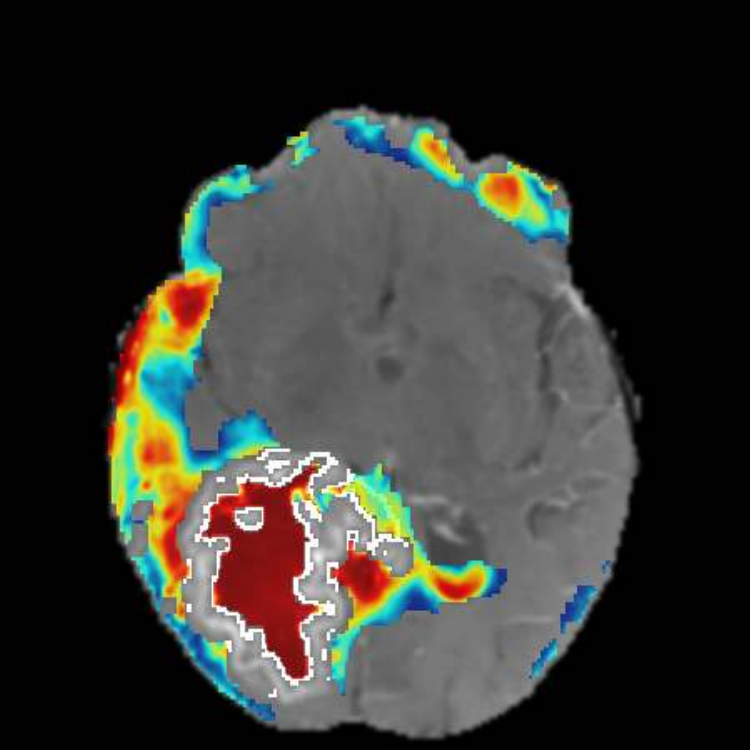} &
		\includegraphics[width=18mm]{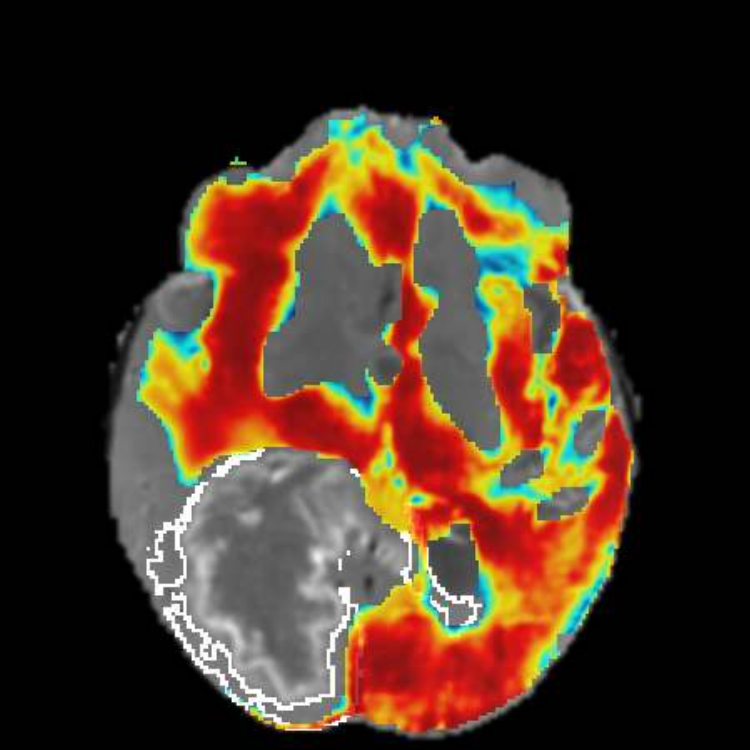} &
		\includegraphics[width=18mm]{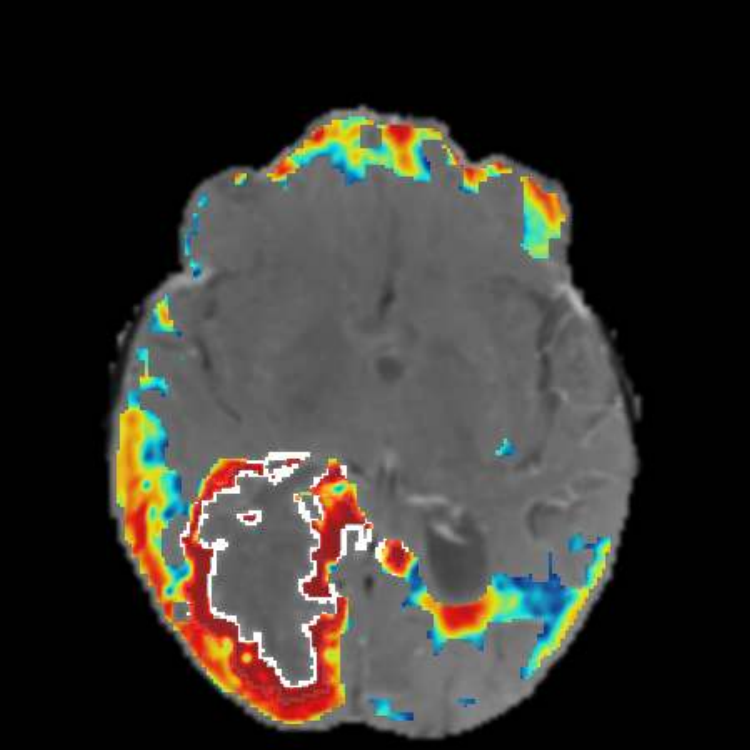} &
		\includegraphics[width=18mm]{figures/figure_4/figure4_19.pdf} &
		\includegraphics[width=27mm, height=18mm]{figures/figure_4/figure4_21.pdf} \\
		\includegraphics[width=18mm,height=17.8mm]{figures/figure_4/figure4w_4.pdf} &
		\includegraphics[width=18mm]{figures/figure_4/figure4_5.pdf} &
		\includegraphics[width=18mm]{figures/figure_4/figure4_6.pdf} &
		\includegraphics[width=18mm]{figures/figure_4/figure4_7.pdf} &
		\includegraphics[width=18mm]{figures/figure_4/figure4_8.pdf} &
		\includegraphics[width=18mm]{figures/figure_4/figure4_9.pdf} &
		\includegraphics[width=18mm]{figures/figure_4/figure4_10.pdf} &
		\includegraphics[width=18mm]{figures/figure_4/figure4_11.pdf} &
		\includegraphics[width=27mm, height=18mm]{figures/figure_4/figure4_20.pdf} \\
		\includegraphics[width=18mm,height=17.8mm]{figures/figure_4/figure4w_12.pdf} &
		\includegraphics[width=18mm]{figures/figure_4/figure4_13.pdf} &
		\includegraphics[width=18mm]{figures/figure_4/figure4_14.pdf} &
		\includegraphics[width=18mm]{figures/figure_4/figure4_15.pdf} &
		\includegraphics[width=18mm]{figures/figure_4/figure4_16.pdf} &
		\includegraphics[width=18mm]{figures/figure_4/figure4_17.pdf} &
		\includegraphics[width=18mm]{figures/figure_4/figure4_18.pdf} &
		\includegraphics[width=18mm]{figures/figure_4/figure4_19.pdf} &
		\includegraphics[width=27mm, height=18mm]{figures/figure_4/figure4_21.pdf} \\
	\end{tabular}
	% {\includegraphics[scale=0.8]{figures/dice_vs_nll.eps}}
	\caption{
		The two bottom rows correspond to two of the cases from the PROMISE12 dataset are marked in (A): Case I and Case II.
	}
	
	\label{fig:dice_vs_nll_more}
\end{figure*}

\begin{figure*}[h]
	% todo: remove vspace later
	%\vspace{-0.6cm}
	\centering
	\setlength{\tabcolsep}{1pt}
	\begin{tabular}{ccc}
		\small{~~~Prostate Segmentation} &
		\small{~~~Brain Tumor Segmentation} &
		\small{~~~Cardiac Segmentation} \\
		\includegraphics[width=58mm]{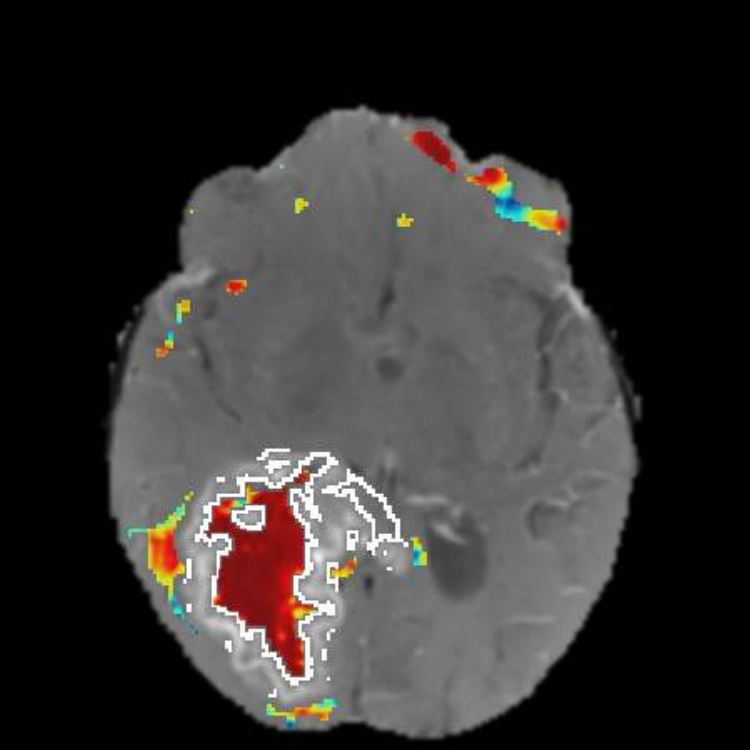} &
		\includegraphics[width=58mm]{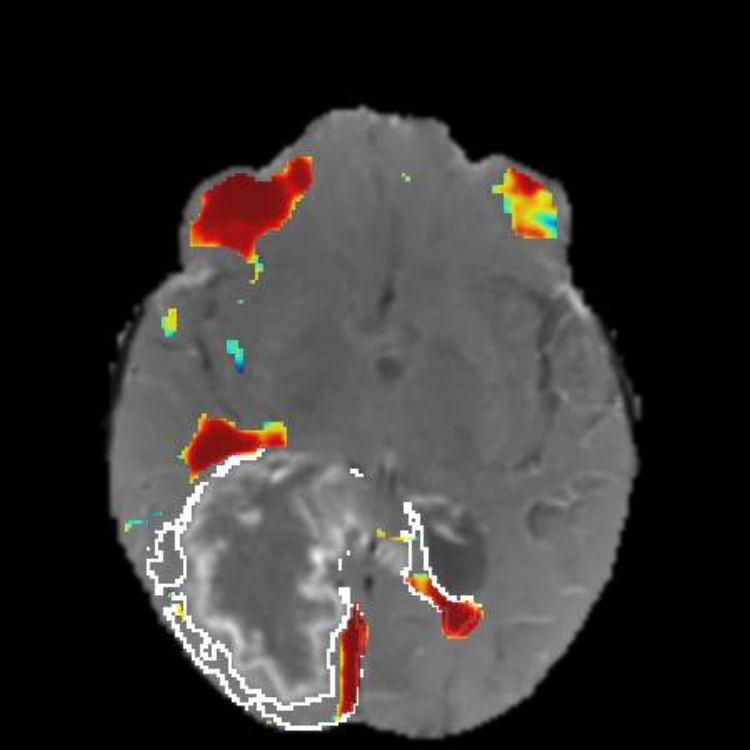} &
		\includegraphics[width=58mm]{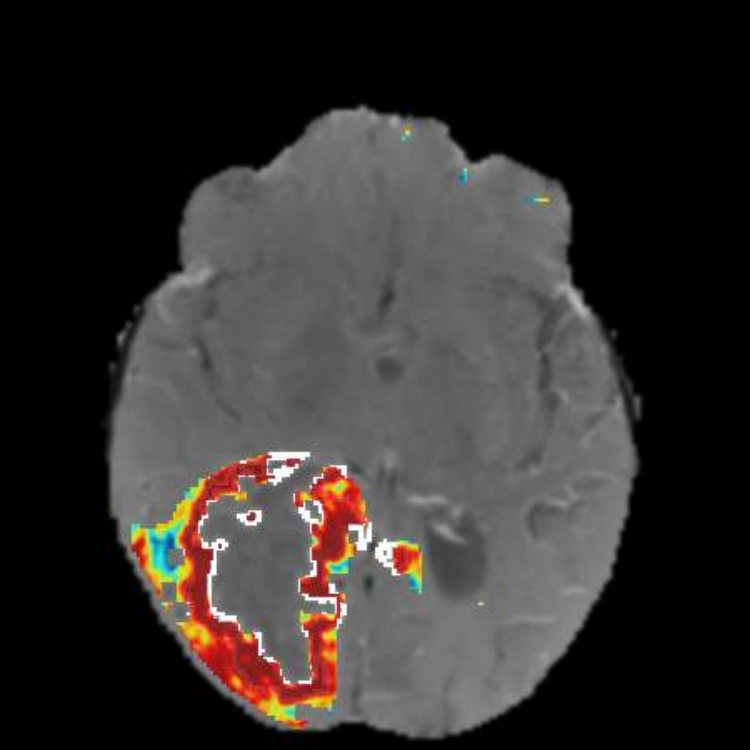} \\

	\end{tabular}
	% {\includegraphics[scale=0.8]{figures/dice_vs_nll.eps}}
	\caption{
		Segment-level predictive uncertainty estimation: Top row: Scatter plots and linear regression between Dice coefficient and average of entropy over the predicted segment .
	}
\label{fig:dice_vs_nll_ce}
\end{figure*}

\clearpage
\newpage
\section{3D FCNs}

Table \ref{tab:confidence_calibration_3d} compares the baselines trained with cross entropy, Dice loss with those calibrated with ensembling and through some representative examples over the three segmentation tasks.
For each prediction map, a reliability diagram over the whole volume is provided.
{\color{lightgray}\blindtext[1]}

\begin{table}[h]
	%\vspace{-0.2cm}
	\centering
	\caption{
		Confidence calibration for baselines trained with Dice loss ($\mathcal{L}_{DSC}$) are compared with those that trained with cross entropy ($\mathcal{L}_{CE}$) and those that were calibrated with ensembling. Bold faced font indicates statistically significant results.} 
	\label{tab:confidence_calibration_3d}
	\begin{tabular}{l|ccc}
		\toprule
		& \multicolumn{3}{c}{Calibration Quality (Bounding Boxes)}\\
		\midrule
		Application (Model) & NLL (95\% CI) & Brier (95\% CI)  & ECE\%  (95\% CI)\\
		\midrule
		Brain ($\mathcal{L}_{DSC}$)& 
		0.14 (0.03$-$0.42)& 0.02  (0.00$-$0.05) & 0.83 (0.17$-$2.50)\\
		Brain (En ${\mathcal{L}_{DSC}}$) & 
		\textbf{0.03 (0.01$-$0.07)} & \textbf{0.01  (0.00$-$0.02)} & \textbf{0.44 (0.02$-$1.33)}\\
		\midrule
		Heart ($\mathcal{L}_{DSC}$)& 
		0.14 (0.03$-$0.42)& 0.02  (0.00$-$0.05) & 0.83 (0.17$-$2.50)\\
		Heart (En ${\mathcal{L}_{DSC}}$) & 
		\textbf{0.03 (0.01$-$0.07)} & \textbf{0.01  (0.00$-$0.02)} & \textbf{0.44 (0.02$-$1.33)}\\
		\midrule
		Prostate ($\mathcal{L}_{DSC}$)& 
		0.14 (0.03$-$0.42)& 0.02  (0.00$-$0.05) & 0.83 (0.17$-$2.50)\\
		Prostate (En ${\mathcal{L}_{DSC}}$) & 
		\textbf{0.03 (0.01$-$0.07)} & \textbf{0.01  (0.00$-$0.02)} & \textbf{0.44 (0.02$-$1.33)}\\
		\bottomrule
	\end{tabular}
	
\end{table}
